# Supplementary material for: Can Dialects Be Steered Like Languages? Sparse Neurons and Distributed Directions in Arabic LLMs
Source: arXiv:2607.03936 source file (2026-09-06)
Supplement: Supplementary file 1 [file MSA2Dialect.tex]

\section{MSA-to-Dialects Steering}
\label{app:msa2dialect}
